# Supplementary material for: Mind's Eye of LLMs: Visualization-of-Thought Elicits Spatial Reasoning in Large Language Models
Source: arXiv:2404.03622 source file (2024-10-23)
Supplement: Supplementary file 1 [file inconsistency-example.pdf]

First, let's look at the target rectangle and identify the empty squares ( ⬜ ):

` ` `

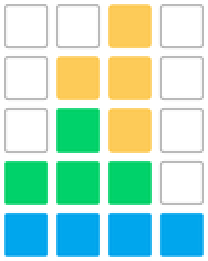

` ` `

We have two polyominoes to fit into this rectangle: Tetromino L ( 🟥 ) and Tetromino I ( 🟪 ). We need to use the variations provided to fill the empty squares without overlapping the existing polyominoes or going outside the rectangle.

Let's start with Tetromino L ( 🟥 ) because it has a unique shape that can fit into corners or protrusions. Looking at the variations of Tetromino L:

Variation 1:

` ` `

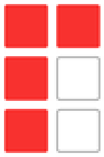

` ` `

Variation 6:

` ` `

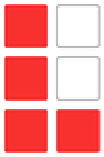

` ` `

We can see that Variation 6 of Tetromino L fits perfectly into the top left corner of the target rectangle, filling three empty squares vertically and turning to fill one horizontally. Let's place Variation 6 of Tetromino L into the target rectangle:

` ` `

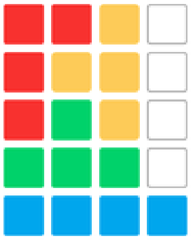

```

Now, we have four empty squares remaining in a straight line, which matches the shape of Tetromino I. Let's look at the variations of Tetromino I:

Variation 1:

```

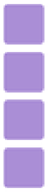

```

Variation 2:

```

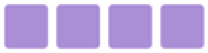

```

Since the remaining empty squares are in a horizontal line, Variation 2 of Tetromino I will fit perfectly. Let's place Variation 2 of Tetromino I into the target rectangle:

```

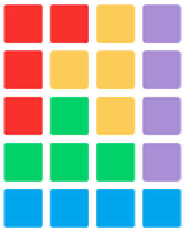

```

The correct variation of Tetromino I that fits into the target rectangle is:

B. 2
```
