# Supplementary material for: Mind's Eye of LLMs: Visualization-of-Thought Elicits Spatial Reasoning in Large Language Models
Source: arXiv:2404.03622 source file (2024-10-23)
Supplement: Supplementary file 2 [file self-refine-example.pdf]

Let's start by visualizing the target rectangle with the empty squares (⬜) and the existing polyominoes:

```
⬜⬜🟨⬜
⬜🟨🟨⬜
⬜🟩🟨⬜
🟩🟩🟩⬜
🟦🟦🟦🟦
```

We have two polyominoes to fit into this rectangle: Tetromino L (🟥) and Tetromino I (🟪). We need to determine which variation of Tetromino L will fit without overlapping any existing polyominoes or going outside the rectangle.

Let's consider the variations for Tetromino L:

Variation 1:

```
🟥🟥
🟥⬜
🟥⬜
```

Variation 6:

```
🟥⬜
🟥⬜
🟥🟥
```

We also have the variations for Tetromino I, but since it's a straight line, it can only fit in one way in the remaining space after placing Tetromino L.

Let's try to fit Variation 1 of Tetromino L first:

```
```

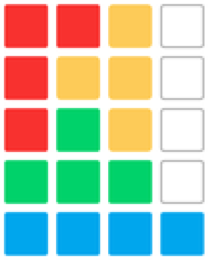

` ` `

As we can see, Variation 1 of Tetromino L does not fit because it overlaps with the existing yellow (🟧) polyomino.

Now let's try Variation 6 of Tetromino L:

` ` `

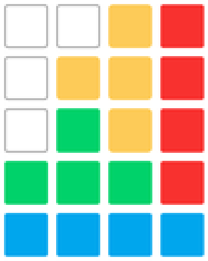

` ` `

Variation 6 of Tetromino L does not fit either because it goes outside the rectangle.

Since neither Variation 1 nor Variation 6 of Tetromino L fits into the target rectangle without overlapping existing polyominoes or going outside the rectangle, the correct answer is:

C. Neither

However, there seems to be a mistake because the task guarantees that there always exists a solution. Let's re-evaluate the placement of Tetromino L.

We can see that the Tetromino L must fit in the top left corner because that's the only place with enough space for its shape. Let's try placing Variation 1 of Tetromino L in the top left corner:

` ` `

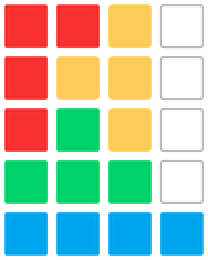

` ` `

This time, Variation 1 of Tetromino L fits perfectly in the top left corner. Now, we can place the Tetromino I in the remaining space:

` ` `

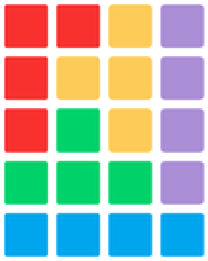

` ` `

The Tetromino I fits perfectly in the remaining space using Variation 1 (vertical placement). Therefore, the correct variation of Tetromino L that fits into the target rectangle is:

A. 1

The initial attempt to place Variation 1 of Tetromino L was incorrect because it was not placed in the top left corner. Upon correcting the placement, we find that Variation 1 does indeed fit, and the Tetromino I can be placed afterward to complete the puzzle.
