# Supplementary material for: Mind's Eye of LLMs: Visualization-of-Thought Elicits Spatial Reasoning in Large Language Models
Source: arXiv:2404.03622 source file (2024-10-23)
Supplement: Supplementary file 3 [file nl-navigation-response.pdf]

Let's visualize the grid with the items you've described:

```
+---+---+---+
| S | B | M |
+---+---+---+
| P | C | V |
+---+---+---+
| T | W | C |
+---+---+---+
```

Where:

- T = Cassette player
- W = Wool
- C = Conch
- V = Moving van
- C = Confectionery store
- P = Pot pie
- S = Siamang
- B = Black-and-white colobus
- M = Minivan

You start at the bottom-left corner where the cassette player is located (T). Now, let's follow your steps:

1. Go right by one step (to Wool - W):

```
+---+---+---+
| S | B | M |
+---+---+---+
| P | C | V |
+---+---+---+
| T | *W* | C |
+---+---+---+
```

2. Go right by one step (to Conch - C):

```
+---+---+---+
| S | B | M |
+---+---+---+
| P | C | V |
+---+---+---+
```

|   |   |   |   |   |     |   |
|---|---|---|---|---|-----|---|
|   | T |   | W |   | *C* |   |
| + | - | - | + | - | -   | + |

3. Go up by one step (to Moving van - V):

|   |   |   |   |   |     |   |
|---|---|---|---|---|-----|---|
| + | - | - | + | - | -   | + |
|   | S |   | B |   | M   |   |
| + | - | - | + | - | -   | + |
|   | P |   | C |   | *V* |   |
| + | - | - | + | - | -   | + |
|   | T |   | W |   | C   |   |
| + | - | - | + | - | -   | + |

4. Go left by one step (to Confectionery store - C):

|   |   |   |     |   |   |   |
|---|---|---|-----|---|---|---|
| + | - | - | +   | - | - | + |
|   | S |   | B   |   | M |   |
| + | - | - | +   | - | - | + |
|   | P |   | *C* |   | V |   |
| + | - | - | +   | - | - | + |
|   | T |   | W   |   | C |   |
| + | - | - | +   | - | - | + |

5. Go left by one step (to Pot pie - P):

|   |     |   |   |   |   |   |
|---|-----|---|---|---|---|---|
| + | -   | - | + | - | - | + |
|   | S   |   | B |   | M |   |
| + | -   | - | + | - | - | + |
|   | *P* |   | C |   | V |   |
| + | -   | - | + | - | - | + |
|   | T   |   | W |   | C |   |
| + | -   | - | + | - | - | + |

6. Go up by one step (to Siamang - S):

|   |     |   |   |   |   |   |
|---|-----|---|---|---|---|---|
| + | -   | - | + | - | - | + |
|   | *S* |   | B |   | M |   |
| + | -   | - | + | - | - | + |
|   | P   |   | C |   | V |   |
| + | -   | - | + | - | - | + |
|   | T   |   | W |   | C |   |
| + | -   | - | + | - | - | + |

7. Go right by one step (to Black-and-white colobus - B):

```

+---+---+---+
| S | *B* | M |
+---+---+---+
| P | C | V |
+---+---+---+
| T | W | C |
+---+---+---+

```

8. Go down by one step (to Confectionery store - C):

```

+---+---+---+
| S | B | M |
+---+---+---+
| P | *C* | V |
+---+---+---+
| T | W | C |
+---+---+---+

```

After following all the steps, you will find yourself at the Confectionery store (C).

Answer: Confectionery store
