# Supplementary material for: Mind's Eye of LLMs: Visualization-of-Thought Elicits Spatial Reasoning in Large Language Models
Source: arXiv:2404.03622 source file (2024-10-23)
Supplement: Supplementary file 4 [file visual-tiling-response.pdf]

Let's start by examining the empty spaces in the target rectangle and the provided polyominoes and their variations. We need to fit the Tetromino I, Tetromino L, and Tetromino T into the empty spaces without overlapping any existing polyominoes or going outside the rectangle.

The target rectangle with 12 empty squares looks like this:

...

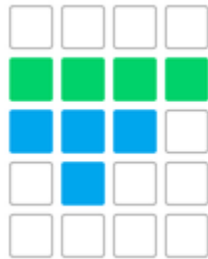

...

We have two variations for Tetromino I (■), which can either be placed vertically or horizontally. Given the configuration of the empty spaces, the only way to place the Tetromino I is horizontally at the top row, as the vertical placement would not fit anywhere.

After placing Tetromino I (■), the target rectangle looks like this:

...

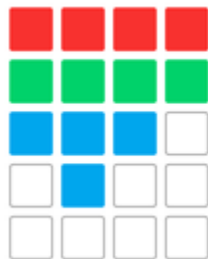

...

Next, we have two variations for Tetromino L (■). We can see that Variation 3 of Tetromino L can fit in the bottom left corner, while Variation 7 would not fit anywhere without overlapping or going outside the rectangle.

After placing Tetromino L (■), the target rectangle looks like this:

...

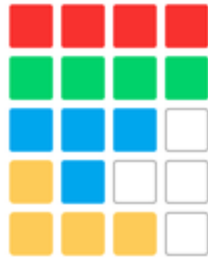

...

Now, we have two variations for Tetromino T ( 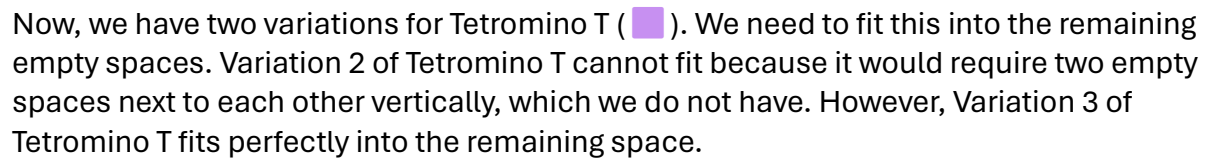 ). We need to fit this into the remaining empty spaces. Variation 2 of Tetromino T cannot fit because it would require two empty spaces next to each other vertically, which we do not have. However, Variation 3 of Tetromino T fits perfectly into the remaining space.

After placing Tetromino T ( 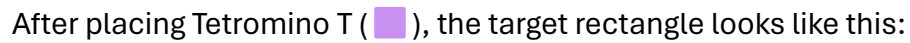 ), the target rectangle looks like this:

...

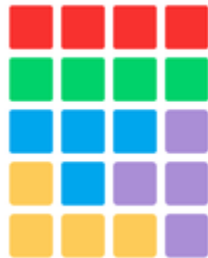

...

The correct variation of Tetromino T that fits into the empty squares is:

B. 3
